# Supplementary material for: Compliant Lattice Modulations Enable Anomalous Elasticity in Ni-Mn-Ga Martensite
Source: arXiv:2407.15181 ancillary file (2024-07-31)
Supplement: Supplementary file 1 [file Supplementary_July_19.pdf]

Supplementary material for

## Compliant lattice modulations enable anomalous elasticity in Ni-Mn-Ga martensite

*Kristýna Repčák<sup>1)</sup>, Pavla Stoklasová<sup>1)</sup>, Tomáš Grabec<sup>1)</sup>, Petr Sedlák<sup>1)</sup>, Juraj Olejňák<sup>2)</sup>, Mariia Vinogradova<sup>3)</sup>, Alexei Sozinov<sup>3)</sup>, Petr Veřtát<sup>4)</sup>, Ladislav Straka<sup>4)</sup>, Oleg Heczko<sup>4)</sup>, Hanuš Seiner<sup>1)</sup>\**

<sup>1)</sup>Institute of Thermomechanics of the Czech Academy of Sciences, Prague 8, 18200, Czech Republic

<sup>2)</sup>Faculty of Nuclear Sciences and Physical Engineering, Czech Technical University in Prague, Prague 2, 12000, Czech Republic

<sup>3)</sup>Material Physics Laboratory, Lappeenranta-Lahti University of Technology (LUT), Lappeenranta, 53850, Finland

<sup>4)</sup>FZU – Institute of Physcs of the Czech Academy of Sciences, Prague 8, 18200, Czech Republic

### S.1 Elastic symmetry of 10 M hierarchically twinned crystals

In this section, we discuss the relation between elastic behaviors of monoclinic single variants of 10 M martensite and of the hierarchical microstructure, and what role this relation plays for the laser-ultrasonic experiments.

#### S.1.1 Theoretical considerations

The coordinate system defined in Figure 1 of the main text aligns the  $c$ -axis of all considered variants (V1, V2, V3, V4) with the axis  $x_2$ , and the  $x_1x_3$  plane is the monoclinic plane. For this reason, the tensor of elastic constants for all these variants can be written formally in the same Voigt's notation form as

$$c_{ij} = \begin{pmatrix} c_{11} & c_{12} & c_{13} & 0 & c_{15} & 0 \\ c_{12} & c_{22} & c_{23} & 0 & c_{25} & 0 \\ c_{13} & c_{23} & c_{33} & 0 & c_{35} & 0 \\ 0 & 0 & 0 & c_{44} & 0 & c_{46} \\ c_{15} & c_{25} & c_{35} & 0 & c_{55} & 0 \\ 0 & 0 & 0 & c_{46} & 0 & c_{66} \end{pmatrix} \quad (\text{S1})$$

having 13 independent elastic constants. The variants differ only in the values of the non-zero components of  $c_{ij}$ , and their elastic tensors can be recalculated from one onto another using symmetry relations (rotations, mirror reflections) between the variants.

In the considered microstructure, the variants are in addition rotated with respect to each other to achieve compatibility. However, because all these four variants share the same  $c$ -axis, all these rotations are rotations about  $x_2$ , and thus, do not alter the structure of the matrix form (S1) of the tensor, changing only the values of the non-zero components.

The microstructure of variants V1-V4 is, however, very particular because of the lattice parameters of 10 M unit cell being very close to tetragonal symmetry. As a result, the variants do not require additional rotations to achieve compatibility over twinning planes (more precisely, less than  $1^\circ$  rotation are needed for all twinning systems between V1, V2, V3 and V4). For this reason, the operation of

$a/b$ -twinning can be very closely approximated just by a mirror reflection over a  $x_2x_3$  plane, while the modulation-twinning operation by mirror reflection over the plane  $x_1=x_3$ . Let us mention that  $1^\circ$  is lower than the typical mosaicity in NiMnGa single crystals, and also comparable with the accuracy with which the orientation can be determined using X-ray diffraction-based methods. From this point of view, the used approximation affects the results less than the expected experimental error.

The symmetry operations representing the  $a/b$  and modulation twinning can be directly applied onto the matrix (S1), which enables us to express the elastic constants of the variants V2 and V3, from those of V1 as follows:

$$c_{ij}^{V2} = \begin{pmatrix} c_{11}^{V1} & c_{12}^{V1} & c_{13}^{V1} & 0 & -c_{15}^{V1} & 0 \\ c_{12}^{V1} & c_{22}^{V1} & c_{23}^{V1} & 0 & -c_{25}^{V1} & 0 \\ c_{13}^{V1} & c_{23}^{V1} & c_{33}^{V1} & 0 & -c_{35}^{V1} & 0 \\ 0 & 0 & 0 & c_{44}^{V1} & 0 & -c_{46}^{V1} \\ -c_{15}^{V1} & -c_{25}^{V1} & -c_{35}^{V1} & 0 & c_{55}^{V1} & 0 \\ 0 & 0 & 0 & -c_{46}^{V1} & 0 & c_{66}^{V1} \end{pmatrix} \quad (S2)$$

and

$$c_{ij}^{V3} = \begin{pmatrix} c_{33}^{V1} & c_{23}^{V1} & c_{13}^{V1} & 0 & c_{35}^{V1} & 0 \\ c_{23}^{V1} & c_{22}^{V1} & c_{12}^{V1} & 0 & c_{25}^{V1} & 0 \\ c_{13}^{V1} & c_{12}^{V1} & c_{11}^{V1} & 0 & c_{15}^{V1} & 0 \\ 0 & 0 & 0 & c_{66}^{V1} & 0 & c_{46}^{V1} \\ c_{35}^{V1} & c_{25}^{V1} & c_{15}^{V1} & 0 & c_{55}^{V1} & 0 \\ 0 & 0 & 0 & c_{46}^{V1} & 0 & c_{44}^{V1} \end{pmatrix}, \quad (S3)$$

and the elastic constants of V4 can be calculated from those of V3 using the same relation as between V2 and V1. Importantly, the same relations hold also between the compliance matrices  $s_{ij}$ , which are matrices inverse to  $c_{ij}$ . Thus, for example, one can write

$$s_{ij}^{V2} = \begin{pmatrix} s_{11}^{V1} & s_{12}^{V1} & s_{13}^{V1} & 0 & -s_{15}^{V1} & 0 \\ s_{12}^{V1} & s_{22}^{V1} & s_{23}^{V1} & 0 & -s_{25}^{V1} & 0 \\ s_{13}^{V1} & s_{23}^{V1} & s_{33}^{V1} & 0 & -s_{35}^{V1} & 0 \\ 0 & 0 & 0 & s_{44}^{V1} & 0 & -s_{46}^{V1} \\ -s_{15}^{V1} & -s_{25}^{V1} & -s_{35}^{V1} & 0 & s_{55}^{V1} & 0 \\ 0 & 0 & 0 & -s_{46}^{V1} & 0 & s_{66}^{V1} \end{pmatrix} \quad (S4)$$

as the relation between the compliance matrices of variants V1 and V2.

For a laminate of two variants, the resulting homogenized elastic constants fall between the so-called *Voigt* and *Reuss estimates*, that give the upper and lower bounds to the effective elastic constants, respectively (Hill, *Proc. Phys. Soc. A*, 65 (1952) 349). If we consider an  $a/b$ -laminate of variants V1 and V2, the Voigt estimate is

$$c_{ij} = \kappa c_{ij}^{V1} + (1 - \kappa) c_{ij}^{V2}, \quad (S5)$$

where  $\kappa$  is the volume fraction of variant V1 in the laminate, while the Reuss estimate is obtained as an inverse matrix to the homogenized compliance matrix

$$s_{ij} = \kappa s_{ij}^{V1} + (1 - \kappa) s_{ij}^{V2}. \quad (S6)$$

It is easily seen that for the orthorhombic part of the tensor (that is,  $c_{11}$ ,  $c_{12}$ ,  $c_{13}$ ,  $c_{22}$ ,  $c_{23}$ ,  $c_{33}$ ,  $c_{44}$ ,  $c_{55}$ , and  $c_{66}$ ) the Voigt and Reuss estimates are independent of the volume fraction  $\kappa$ , and are identical to each other, which means also identical to the corresponding elastic constants of a single variant. In other

words, independent of the volume fractions of the variants, the experiments performed on a V1:V2 laminate enable direct determination of single-variant monoclinic elastic constants except for  $c_{15}$ ,  $c_{25}$ ,  $c_{35}$ , and  $c_{46}$ . These four constants vanish to zero if  $\kappa = 0.5$ , for which the microstructure attains mirror symmetry over the  $a/b$  twinning plane.

For the twins-within-twins hierarchical microstructure involving all variants, the Voigt estimate reads

$$c_{ij} = \kappa_1 c_{ij}^{V1} + \kappa_2 c_{ij}^{V2} + \kappa_3 c_{ij}^{V3} + \kappa_4 c_{ij}^{V4}, \quad (S7)$$

and the Reuss estimate can be calculated from

$$s_{ij} = \kappa_1 s_{ij}^{V1} + \kappa_2 s_{ij}^{V2} + \kappa_3 s_{ij}^{V3} + \kappa_4 s_{ij}^{V4}, \quad (S8)$$

where  $(\kappa_1 + \kappa_2 + \kappa_3 + \kappa_4) = 1$  are the volume fractions of the respective variants.

In this case, the Voigt and Reuss estimates meet only for two elastic constants,  $c_{33}$  and  $c_{55}$ , and for these constants the estimates are also equal to  $c_{22}$  and  $c_{55}$  for the monoclinic single variant. This means that measurements of the effective elastic constants of this type of microstructure enables only determination of these two constants of the single variant.

### S.1.2 Implications for laser-ultrasonic measurements

As explained in the main text, the TGS experiments were performed on an  $a/b$ -laminate, including a pair of variants sharing the same orientation of modulation, such as for example the variants V1 and V2. As explained above, if the 13 monoclinic elastic constants of such a laminate were measured, the orthorhombic part of the resulting tensor would be equal to the orthorhombic part of the monoclinic elastic tensor of a single variant.

In the experiments, we observed clear mirror symmetry of the TGS maps with respect to the principal planes, which meant that the non-orthorhombic constants  $c_{15}$ ,  $c_{25}$ ,  $c_{35}$ , and  $c_{46}$  of the analyzed laminate were very close to zero. This might have been either because the volume fraction in the laminate was close to  $\kappa = 0.5$ , or because these constants are very small even for the single variant itself (as also indicated by DFT calculations ([Seiner et al. Phys. Status Solidi RRL 16 \(2022\) 2100632](#))). The latter explanation is quite plausible, because of the very small deviation of the symmetry of the unit cell from mirror symmetries with respect to the principal planes. Let us point out that the shape of the unit cell is approximately tetragonal ( $a \approx b$ , monoclinic angle  $\gamma \approx \pi/2$ ), but the presence of the modulation breaks the four-fold axis and reduces the resulting symmetry to approximately orthorhombic. Regardless of the reason for this additional symmetry, the orthorhombic elastic tensor determined from TGS maps includes, based on the analysis above, elastic constants of a single variant.

In the RUS measurements performed on the twin-within-twins second-order laminate, the expected effective elastic anisotropy should be monoclinic, because of mixing behaviors of two (monoclinic or orthorhombic)  $a/b$ -laminates. The above theoretical analysis shows that such monoclinic elastic tensor includes  $c_{22}$  and  $c_{55}$  equal to those of a single variant, while all other variants are dependent on the volume fractions  $\kappa_1$ ,  $\kappa_2$ ,  $\kappa_3$ , and  $\kappa_4$ . However, as discussed for example in ([Landa et al. Appl. Phys. A 96 \(2009\) 557](#)), the RUS measurements are dominantly sensitive only to the softest elastic constants or their softest combinations. If the anisotropy is extremely strong, such as in the case of 10 M NiMnGa martensite, several tens of the lowest resonant frequencies of the sample are nearly independent of all other elastic constants but the softest one. The RUS spectra obtained on the examined sample were strongly damped, which enabled us to detect and identify less than 20 peaks. Using the sensitivity analysis described in ([Sedláč et al. Exp. Mech. 54 \(2014\) 1073](#)), we confirmed that for the range of  $c_{55}$  estimated from the TGS experiments (i.e., between 0.4 GPa and 6.5 GPa), these resonant frequencies were nearly fully determined by  $c_{55}$  only.

This allowed us to determine the effective  $c_{55}$  of the laminate, and entitles us to interpret the obtained value of  $c_{55} = 2.1$  GPa as the average constant of  $c_{55}$  of a single variant averaged over the whole volume of the sample.

## S.2 XRD experiments

X-ray diffraction (XRD) experiments presented in this Supplementary material were performed using a PANalytical X'Pert PRO diffractometer with a Co anode in a Bragg-Brentano geometry. We used point focus and ATC-3 texture cradle serving as a sample goniometer allowing us to study reciprocal space from a bulk single crystal sample. The cradle limited the maximal  $2\theta$  angle to  $\sim 130^\circ$ .

The beam footprint was defined by a fixed  $0.25 \times 1$  mm collimator (vertical  $\times$  horizontal). The actual footprint on the sample surface was approximately  $(3.7 - 1.1) \times 1.7$  mm<sup>2</sup> (length  $\times$  width; with the first length value representing the upper limit for  $2\theta = 30^\circ$  and the second length value the lower limit for  $\theta = 130^\circ$ ).

The lattice parameters of our slightly monoclinic unit cell were previously established as follows:  $a = 5.961$  Å,  $b = 5.943$  Å,  $c = 5.601$  Å,  $\gamma = 90.31^\circ$  through the high-resolution XRD measurements of the (400), (040), (004), (600), (060), (006), (440), (620), (260), (404), (044), (-440), (602), and (062) reflections.

### S.2.1 Confirmation of commensurate 10 M martensite structure

For correct interpretation of the results from laser-ultrasonic measurement, we first confirmed the 10 M modulated martensite structure at room temperature. Before conducting the measurement, the sample microstructure was favourably reoriented, with  $a$ - and  $b$ - axes pointing out of plane (both were present due to the  $a/b$  twinning).

Then we measured a  $hk0$  reciprocal space map (RSM) containing (220), (400) and (440) strong reflections, along with their modulation satellites in the  $[110]^*$  direction, [Supplementary Figure 1](#). The RSM was acquired at the midpoint of the sample. The presence of *modulation twins* resulted in the revelation of a second twin domain with satellites observed apparently in the  $[-110]^*$  direction. These satellites exhibited even greater intensity compared to those in the  $[110]^*$  direction.

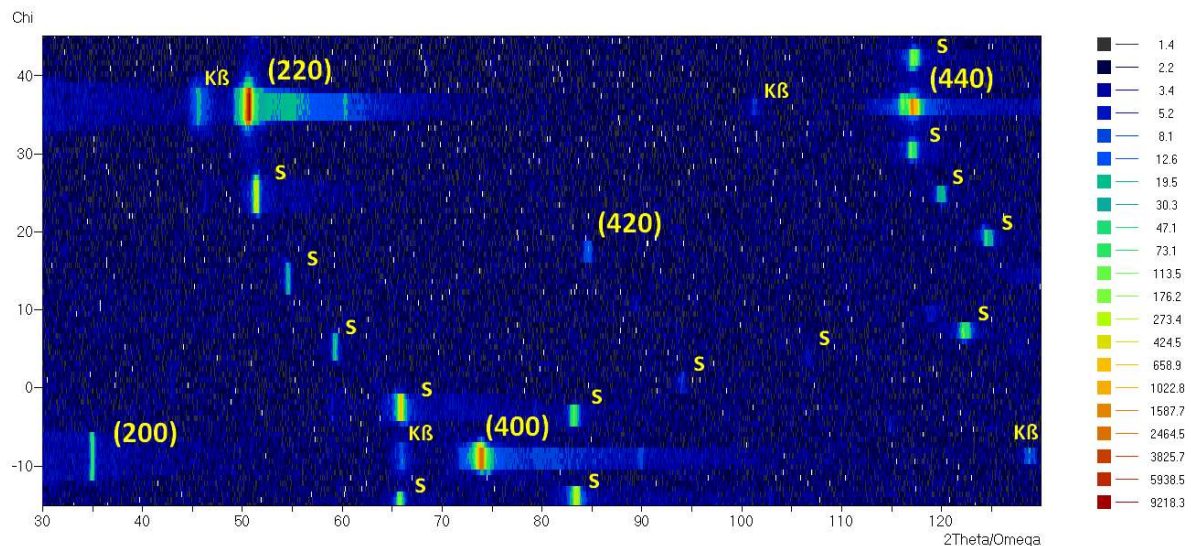

[Supplementary Figure 1](#):  $(hk0)$  reciprocal space map in instrumental coordinates from the midpoint of the sample. Satellite reflections are marked by "s". The absence of monochromator resulted in minor contribution from the  $K_\beta$  line (marked in the figure) and noticeable tube tails.

It is important to note that the reflection (220) marked in the map may in fact correspond also to the (-220), (-2-20) and/or (2-20) reflections that may be present due to twinning. Similarly, within the spot marked (400), both (400) and (040) reflections coexist. Due to the optics employed with the absence of monochromator, these reflections cannot be easily resolved from the presented RSM. Nevertheless, used approach is fully suitable for confirmation of 10 M structure. Using higher resolution, unfortunately, would significantly reduce the overall intensity.

For a straightforward interpretation, the measured RSM recalculated into reciprocal coordinates is presented in [Supplementary Figure 2](#). The observed pattern distinctly aligns with the characteristic diffraction pattern expected for the 10M martensite.

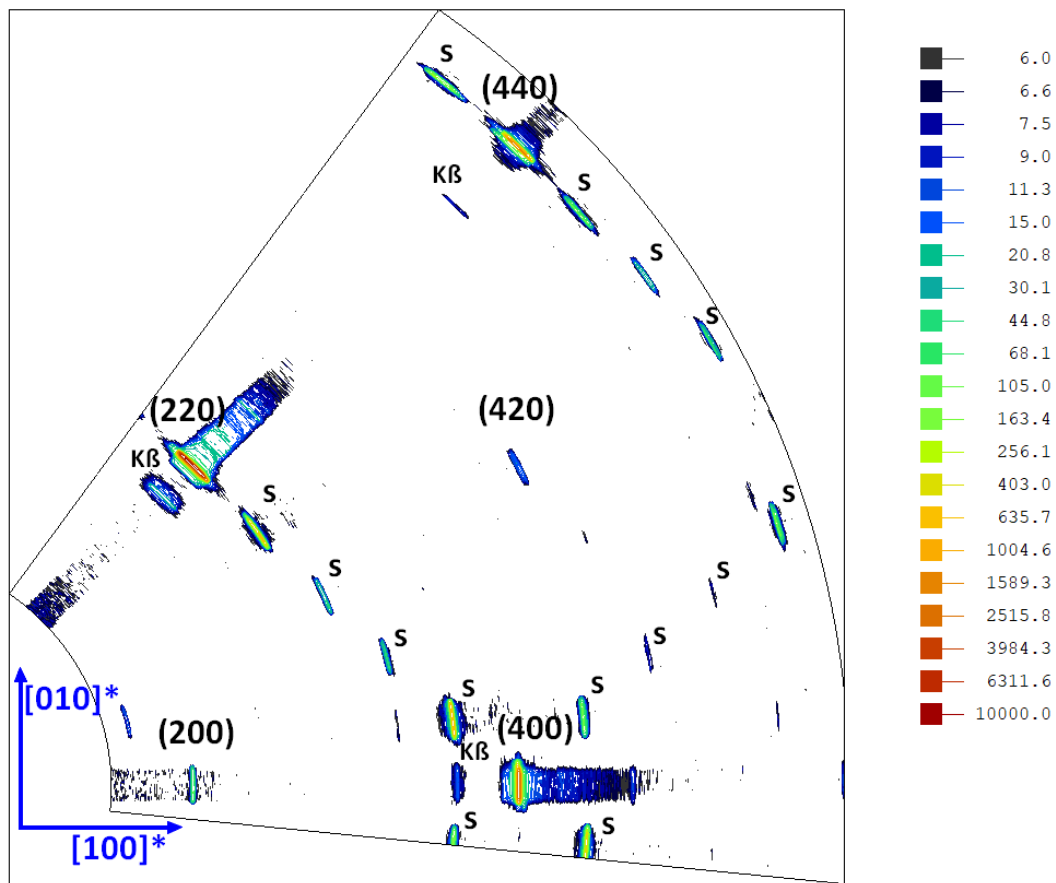

**Supplementary Figure 2:**  $(hk0)$  reciprocal space map converted from [Supplementary Figure 1](#) into reciprocal coordinates. Observed pattern indicate the 10M modulated martensite. Satellite reflections are marked "s". The absence of monochromator resulted in minor contribution from the  $K_\beta$  line (marked in the figure) and noticeable tube tails.

Based on the positions of the satellite reflections, we determined the modulation vector as  $\mathbf{q} = (0.399(2), 0.399(2), 0)$ , approximately equivalent to commensurate  $(2/5, 2/5, 0)$ . The slightly larger error is attributed to lower resolution in  $2\theta$  and defocusing induced by the necessary sample tilt in our experimental setup. No additional low-intensity satellites, indicative of incommensurate modulation ([Veřtát et al., J. Phys. Condens. Matter 33 \(2021\) 265404](#)), were detected, providing additional confirmation of the commensurate (or at least nearly commensurate) state.

The distribution of *modulation twin domains* exhibited variation along the sample, as illustrated in [Supplementary Figure 3](#) representing the RSM measured at the different location on the sample surface (the end of the sample instead of the midpoint). In contrast to [Supplementary Figure 1](#),

satellites in the  $[110]^*$  direction (highlighted red in the figure) are now stronger than those in the  $[-110]^*$  direction.

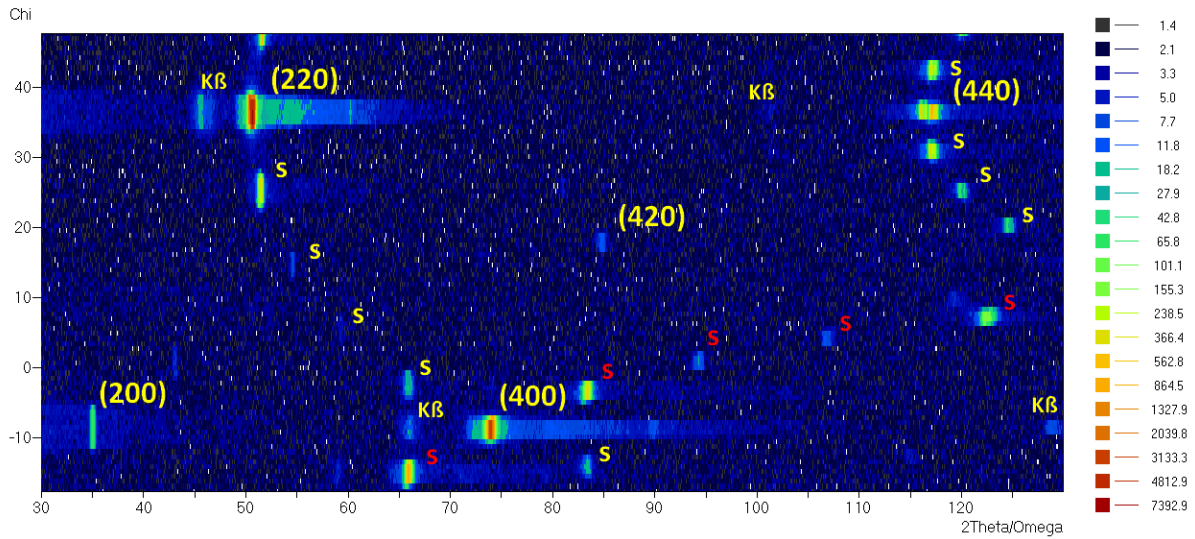

**Supplementary Figure 3:**  $(hk0)$  reciprocal space map in instrumental coordinates from the end of the sample. Satellites in the  $[110]^*$  direction are highlighted red for clarity.

Despite the varying distribution of twin domains, the diffraction pattern once again distinctly aligned with the characteristic commensurate 10M martensite structure. We determined the modulation vector as  $\mathbf{q} = (0.402(2), 0.402(2), 0)$ , equivalent to  $(2/5, 2/5, 0)$  within experimental error.

### S.2.2 Establishing the direction of the modulation from the $c$ -oriented sample used for final measurements

The laser-ultrasonic measurements necessitated the reorientation of the sample, positioning the  $c$ -axis out of the plane. This posed a significant complication for the diffraction analysis, as the most favorable  $(hk0)$  plane for easy straightforward evaluation of the modulation twins was not accessible with our experimental setup. Therefore, to analyse the presence of satellites in the  $[110]^*$  or  $[-110]^*$  direction, in other words to analyse the presence of  $(V1+V2)$  vs.  $(V3+V4)$  variants, we measured the  $(hhl)$  reciprocal space map, with a focus on the reflection  $(004)$  and its extremely weak modulation satellites in the  $[110]^*$  or  $[-110]^*$  directions. Measured RSM in instrumental coordinates is presented as [Supplementary Figure 4](#) with marked fundamental reflections. Despite the anticipated weak intensity, the first-order modulation satellites associated with the  $(004)$  reflection were distinctly detected, indicating the presence  $(V1+V2)$  twin variants. For straightforward interpretation, the measured RSM recalculated into reciprocal coordinates is presented in [Supplementary Figure 5](#). It confirms that the detected modulation satellites are indeed along the  $[110]^*$  direction and their position corresponds to the aforementioned modulation vector.

To examine the presence of the second domain (*modulation twin*,  $(V3+V4)$  variants, manifested by satellites in  $[-110]^*$  direction in previously presented  $(hk0)$  RMSs), we rotated the sample  $90^\circ$  around its  $c$ -axis and measured RSM analogous to that in [Supplementary Figure 4](#). In the resulting map, [Supplementary Figure 6](#) and [Supplementary Figure 7](#), the  $(004)$  and  $(-224)$  reflections were clearly visible, but there were no satellites found. This ruled out the presence of the  $(V3+V4)$  variants and confirmed the singular direction of modulation within the analyzed volume of the sample.

As a proof of concept, we replicated the same measurements at the end of the sample, where the optical microscopy revealed several modulation macro-twin bands. In this scenario, the presence of satellites was detected in both cases ( $[110]^*$  and  $[-110]^*$  directions), indicating the standard presence of both *modulation twin domains*, i.e. all four (V1-V4) variants.

In summary, the XRD experiments confirmed that in the locations where the TGS measurements were performed, the material was an *a/b*-twinned 10 M martensite with a single orientation of the modulation (this orientation was set as the  $x_1$ -axis for the elastic coefficients) and with approximately commensurate modulations.

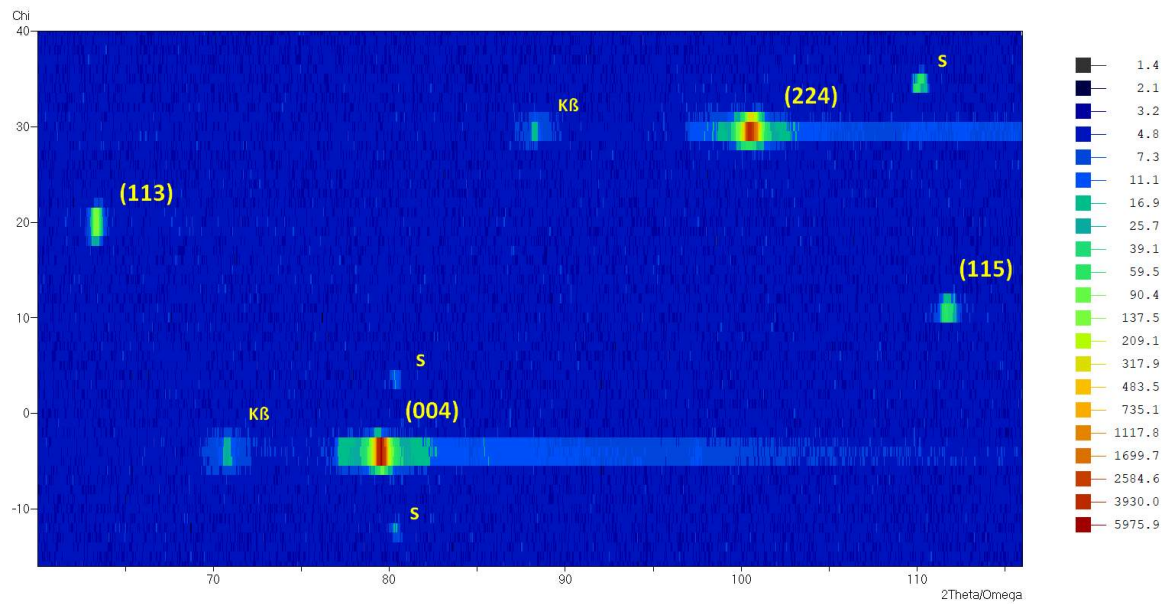

Supplementary Figure 4: (*hkl*) reciprocal space map in instrumental coordinates. The measurement distinctly reveals two modulation satellites around the (004) reflection in the  $[110]^*$  direction, both denoted as "s." For the recalculated map into reciprocal coordinates, refer to Fig.XRD.5.

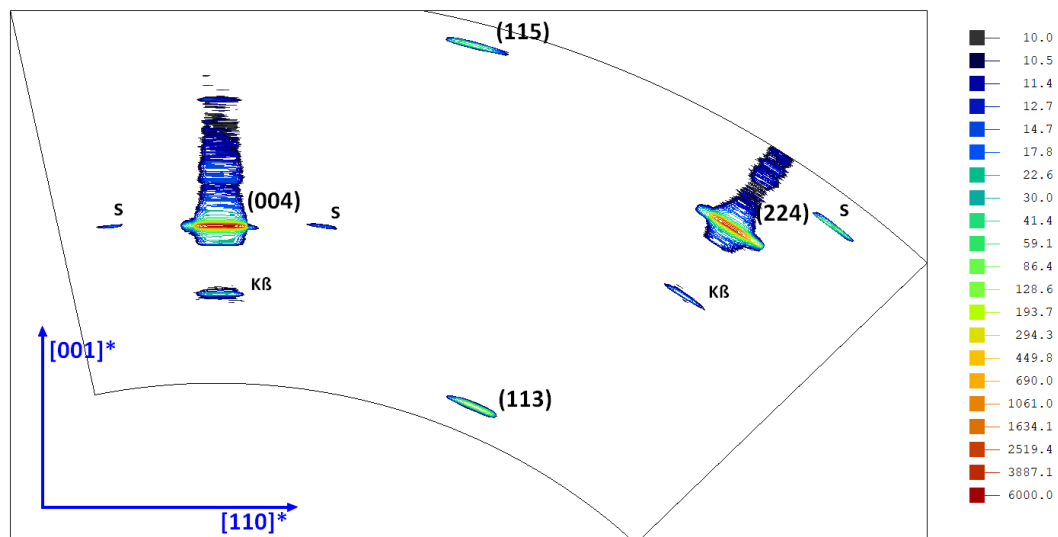

Supplementary Figure 5: (*hkl*) reciprocal space map converted from Supplementary Figure 4 into reciprocal coordinates, highlighting the presence of modulation satellites of the (004) reflection in the  $[110]^*$  direction.

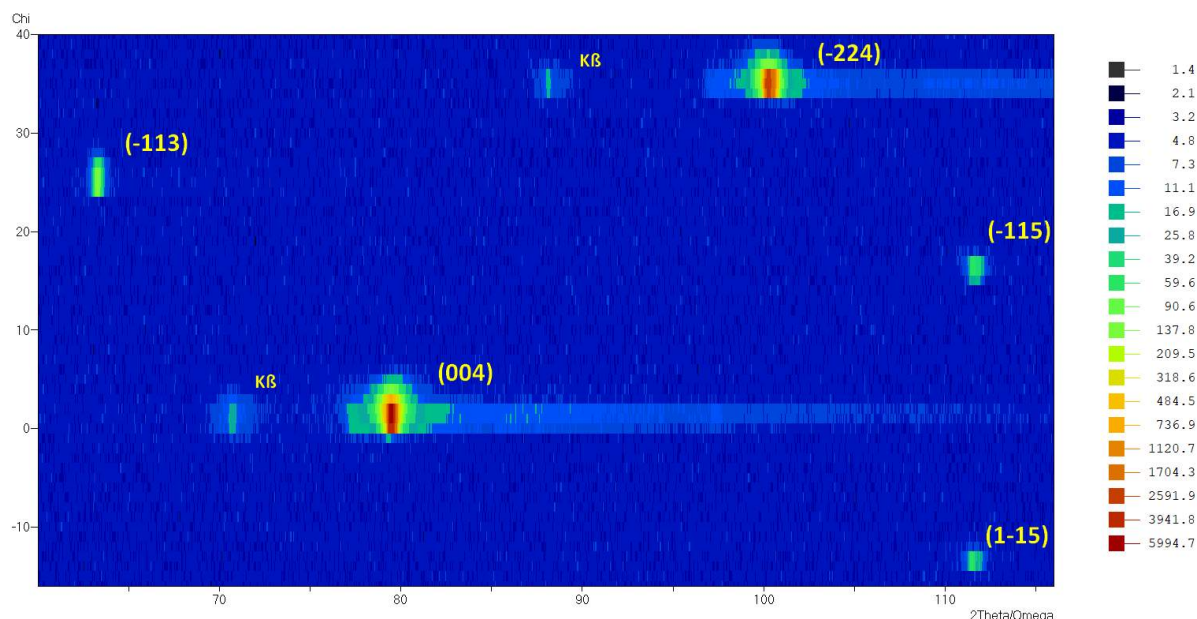

Supplementary Figure 6:  $(-hhl)$  reciprocal space map in instrumental coordinates indicating the absence of the modulation satellites around the (004) reflection in the  $[-110]^*$  direction. For recalculated map into reciprocal coordinates, see Supplementary Figure 7.

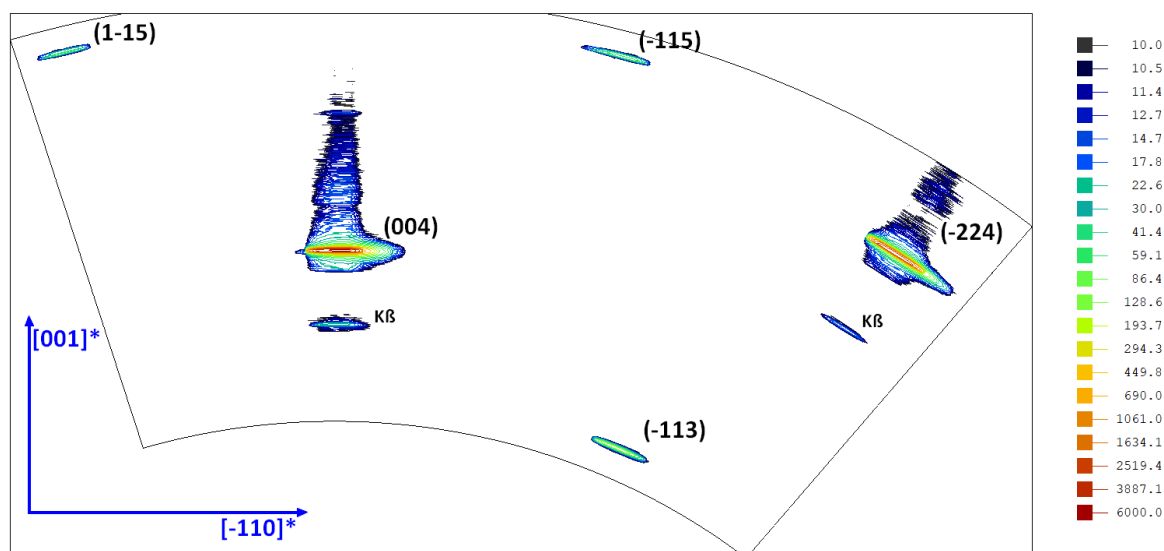

Supplementary Figure 7:  $(-hhl)$  reciprocal map converted from Supplementary Figure 6 into reciprocal coordinates. No visible satellite reflections were detected in the  $[-110]^*$  direction.

### S.3 Discussion of heterogeneity and softness in $c_{55}$ : the effect of $a/b$ -twins and the modulation vector

As shown in section S.1 of this Supplementary material, the different  $a$ - and  $b$ -lattice orientations within  $a/b$  laminates do not preclude determination of single-variant elastic constants within the orthorhombic part of the tensor. In particular, the extremely soft  $c_{55}$  coefficient is the same for both possible orientations, and is also invariant with respect to the modulation-twinning operation, which

means that it can be directly assessed through RUS measurements on the hierarchically twinned crystal. However, the presence of  $a/b$ -twins as defects in the lattice can still affect its elastic response.

The first possible mechanism is by the motion of the twin boundaries back and forth under the action of the traveling shear wave. Even a local or partial motion (such as by a sideways glide of twinning dislocations along the twin boundaries) might have a softening effect. Importantly, the shear carried by the  $a/b$  reorientation is the  $c_{55}$ -related shear, which means that the soft elastic constant and the reorientation are closely interconnected. As shown in (Kustov et al., *Scripta Mater.* 178 (2020) 483),  $a/b$  twins may indeed be set into motion at frequencies close to 100 kHz. This is clearly demonstrated by the amplitude-dependent elastic response and damping reported. Nevertheless, the TGS measurements operate at much higher frequencies (100 MHz), and the amplitudes are well below  $10^{-6}$ , which is approximately the limit for activating the motion, at least from the experiments reported in (Kustov et al., *Scripta Mater.* 178 (2020) 483). Also, the RUS measurements (at  $\sim 100$  kHz) give a consistent result with TGS, which means there is no frequency-dependence in the  $c_{55}$ , and which also indicates that the motion of  $a/b$  twin boundaries is not the primary source of the very strong anisotropy.

On the other hand, the  $a/b$ -twin boundaries motion is, in fact, equivalent to modifying the stacking sequence. The change of the sequence from  $3/-2/3/-2$  to  $2/-3/2/-3$ , which constitutes the  $a/b$ -twin reorientation, utilizes the same mechanism as the relaxation of shear strains discussed in Figure 3 of the main text. From this point of view, the relation between  $a/b$  twinning and the soft  $c_{55}$  definitely exists, and might be well understood in a reversed sense: it is not the motion of the  $a/b$  twins that results in the low value of measured  $c_{55}$ , but it is rather the instability of the lattice with respect to faulting the sequence (seen as soft  $c_{55}$  in the experiment) that enables easy motion of the  $a/b$  twin boundaries.

The second possible mechanism is that the  $a/b$  twins, as defects in the lattice, might stiffen or soften locally the elastic response by affecting the distances and bonds between the atoms. A similar effect has been theoretically predicted for NiTi (Wang and Sehitoglu, *Int. J. Plast.* 61 (2014) 17), and later also experimentally confirmed (Grabec et al., *Acta Mater.* 208 (2021) 116718). For Ni-Mn-Ga, first-principles calculations (Gruner et al., *Sci. Rep.* 8 (2018) 8489) predict that when two stacking sequences meet at an  $a/b$  twin as  $3/-2/3/-2//2/-3/2/-3$ , the  $-2/2$  pair in the middle leads to local energy reduction (stabilization), while when they meet creating a  $3/-3$  pair, i.e.  $3/-2/3/-2/3//2/-3/2/-3/2$ , the energy becomes locally increased and the defect is unstable. This may, in principle lead to heterogeneity in the elastic constants because of heterogeneous density of  $a/b$  twins (S. Fähler, *personal communication*, 2023). The temperature-resolved elasticity measurements reported in (Veřtát et al., *J. Phys. Condens. Matter* 33 (2021) 265404) show that when the microstructure changes from commensurate to incommensurate due to a temperature cycle, the elastic constants significantly stiffen. Thanks to the hysteretic behavior of the modulation vector, one can compare room temperature stiffness of the material in the commensurate condition and the incommensurate condition, where the former is much softer. Since the incommensurate structure typically exhibits a higher density of  $a/b$  twins than the commensurate structure (Veřtát et al., *J. Phys. Condens. Matter* 33 (2021) 265404), this observation may indicate that  $a/b$  twins are stiffening the lattice, which would be an opposite effect to the softening due to twin boundary motion discussed above.

To elucidate the role of the  $a/b$  twins experimentally, additional TGS experiments were performed on another Ni-Mn-Ga single crystal, from which the  $a/b$  twins were removed by pre-stress. The sample was glued onto a linear mechanical stage enabling pulling the material gently along a direction perpendicular to the  $c$ -axis (the  $c$ -axis and the pulling direction were both set parallel to the studied face of the sample). Because of the chosen crystal orientation and the very low  $a/b$  reorientation stress, this pulling enabled driving out most of the  $a/b$  twins from the sample. The pre-stressed sample was then studied by TGS. Angular frequency maps were recorded in two different locations, with the

aim to explore whether the absence of the  $a/b$  twins leads either to stiffening of  $c_{55}$  towards the values comparable to those predicted by ab-initio calculations (see Table 1 in the main text), or to removing the heterogeneity in the  $c_{55}$  behavior over the volume of the sample.

The results are shown in [Supplementary Figure 8](#). It is seen that the maps are topologically very similar to those reported for stress-free Ni-Mn-Ga in the main text (cf. the experimental and calculated contours in the lower row of Figure 2 in the main text, mind the angular shift resulting from the different geometry of the sample). This already indicates that the removal of  $a/b$  twins does not significantly affect the strength or character of elastic anisotropy. In more detail, it is seen that the minima on the S-wave contours, representing the soft  $c_{55}$  constants, are also present in both maps, and have different depths. Rough estimates of the values were obtained by assuming that all other elastic constants are the same as for the material reported in the main text. This resulted in  $c_{55} = 5.5$  GPa for the first location, and  $c_{55} = 6.1$  GPa in the second location, which falls within the ranges reported in the main text for stress-free Ni-Mn-Ga. In general, one can expect  $c_{55}$  to be slightly higher in the pre-stressed sample, because pulling along the  $a$ -axis stabilizes the material against lowering the tetragonal distortion (the  $a/c$  ratio), which means such a mechanical loading is equivalent to cooling the material down, further away from reverse transition temperature, and thus increasing, its stability. Let us note that such a stabilization might be induced also by the magnetic field, and that may be why ([Dai et al. , J. Appl. Phys. 95 \(2004\) 6957](#)) observed the lowest shear coefficients (equivalent to  $c_{55}$  on a hierarchically twinned sample) being  $c^* \approx 5$  GPa at minimum, instead of 2 GPa as obtained from our RUS experiment, although the material was very similar.

Despite this general increase, it can be clearly concluded that  $c_{55}$  in the material without  $a/b$  twins is comparable to that with  $a/b$  twins (and much smaller than what the ab-initio calculations predict), and that some heterogeneity in the  $c_{55}$  behavior is preserved. That is, the  $a/b$  twins cannot be identified as a primary source of these phenomena.

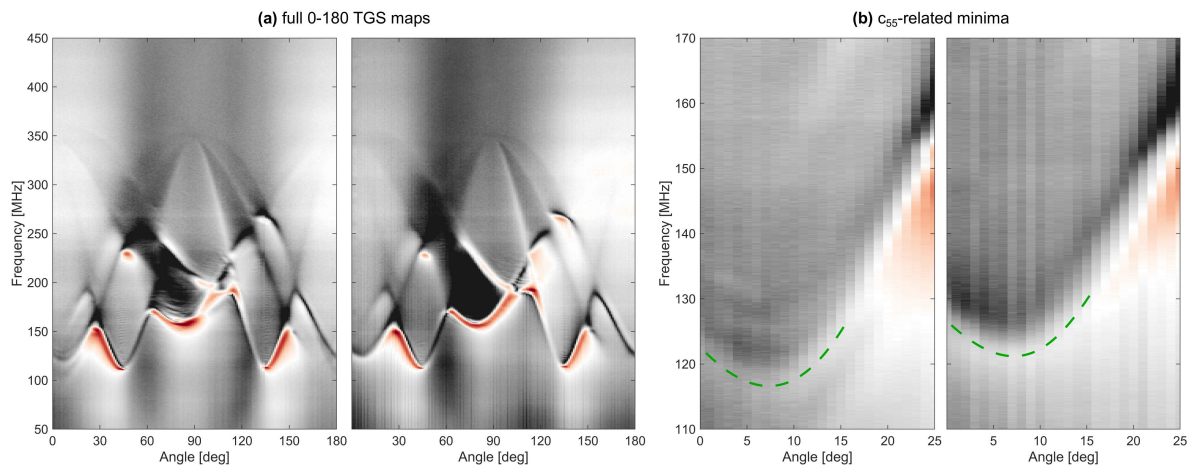

**Supplementary Figure 8:** TGS maps (plots of FFT amplitude with respect to frequency and direction) for a Ni-Mn-Ga sample with  $a/b$ -twins being removed by uniaxial tension, aligning the long  $a$ -axis along the tension direction. The measurements were performed in two different locations, being on the left and on the right in each subfigure, respectively. (a) shows the full maps, that are merely identical; (b) shows details of the S-wave close to the principal direction, where the minimum determines the value of  $c_{55}$ . The green dashed lines are guides for eye, approximating the maxima of the S-wave peaks near the minimum. The minimum frequencies are 116 MHz (estimated  $c_{55} = 5.5$  GPa) for the first location, and 122 MHz (estimated  $c_{55} = 6.1$  GPa) for the second.

As mentioned in the main text, there might be various reasons other than the  $a/b$ -twins why the elastic relaxation through reversible faulting of the stacking sequence can be locally blocked: defects, chemical heterogeneities, mosaicity, internal stresses. With the generalized Zener anisotropy ratio of  $A^* = 255$ , the lattice is, indeed, highly unstable, and may exhibit a strong tendency to rearrange locally into more stable configurations.

Very probably, this also has a direct relation to the stiffening of 10 M martensite with cooling, reported in (Veřtát et al., *J. Phys. Condens. Matter* 33 (2021) 265404). The stiffening reflects the evolution of the modulations from commensurate to incommensurate, and is accompanied with narrowing of the resonant peaks, indicating a decrease in the internal friction coefficients, as well as with turning the character of vibrations from nonlinear to linear (see Figures 7, 8, and 9 in (Veřtát et al., *J. Phys. Condens. Matter* 33 (2021) 265404)). All these features may be interpreted as an evidence of suppressing the inelastic phenomena. The incommensurateness (i.e., the modulation vector of  $q \neq 2/5$ ) indicates pre-existing faults in the sequence, and since these faults appear gradually on cooling, they can be understood as stabilizing the structure against easy reversible faulting needed for the low- $c_{55}$  behavior. Similarly as for the dynamic faulting of the sequences itself, capturing the effect of the incommensurateness on the elastic constants by first-principles calculations would be quite challenging, because very large computational supercells would need to be used to allow for small changes of the modulation vector.
